# Supplementary material for: Exploratory Hidden Markov Factor Models for Longitudinal Mobile Health Data: Application to Adverse Posttraumatic Neuropsychiatric Sequelae
Source: arXiv:2202.12819 source file (2023-06-05)
Supplement: Supplementary file 1 [file 2_additional_data.tex]

In this paper, we consider a subset of the AURORA data by selecting patients involved in MVC before presenting to the ED to investigate the dynamic change in patients' mental health conditions in the $100$ days following MVC exposure. We maintain only observations with no missing data and a positive wake percentage when looking at the activity data. In terms of heart rate data, each individual is anticipated to have $2880$ records every day. In mobile health data, however, missing data is widespread. We keep only observations on days with more than $30\%$ $(2880*0.3)$ recordings to derive representative daily summary statistics.

Prior to fitting our model, we further use the Box-Cox transformation \citep{osborne2010improving} on each variable to reduce the skewness of the original data, delete extreme values and scale the data by dividing the sample standard deviation for each variable. %remove highly-correlated features,

The final dataset we used included observations collected from $258$ patients, each having a different number of total daily records ranging from $17$ to $99$. Note that observations in this dataset are irregularly sampled. Therefore, a subset of it, including only observations collected at \{day $2$, day $12$, $\cdots$, day $82$\}, is also of our interest. In the subset with systematic observations, $180$ patients are included. 

Based on domain knowledge, $23$ variables are of our main interest. Four of them are derived from the activity data, while the remaining $19$ are derived from the HRV data (i.e, {meanAcc}, {amplitude}, {SWCK}, {L5}, {NNmean.min}, {NNmean.mean}, {NNskew.q3}, {SDNN.max}, {SDNN.min}, {SDNN.mean}, {SDNN.var}, {lfhf.min}, {lfhf.mean}, {dc.min}, {dc.mean}, {SD1SD2.max}, {SD1SD2.min}, {SD1SD2.mean}, {SD1SD2.var}, {ApEn.max}, {ApEn.min}, {ApEn.mean}, {ApEn.var}). Besides, the transition model includes both {age} (range from $18$-$74$) and {gender} ($0$-male, $1$-female) to investigate the effect of age and gender on the transition probabilities.
